# Supplementary material for: Breaking the Bias: Recalibrating the Attention of Industrial Anomaly Detection
Source: arXiv:2412.08189 source file (2024-12-11)
Supplement: Supplementary file 1 [file 6_appendix.tex]

\clearpage
\setcounter{page}{1}
\maketitlesupplementary

\section{Inference Speed, GPU Memory, and Model Parameters}
In Table~\ref{appendix_tab1}, the impact of different post-training quantization methods and bit widths on the Inference Speed, GPU Memory, and Model Parameters is demonstrated.

\begin{table}[!ht]
\centering

\setlength\tabcolsep{6pt}
    \begin{tabular}{c|cccc}
    \toprule[1.0pt]
    {Method} & {W/A} & {FPS} & {Mem(MB)} & {Params(M)} \\ \hline 
    {baseline} & {32/32} & \multicolumn{1}{c}{{167}} & {30.7} & {8.05} \\ \hline
    {} & {2/2} & \multicolumn{1}{c}{{147}} & {30} & {0.5} \\
    {} & {3/3} & \multicolumn{1}{c}{{147}} & {30} & {0.75} \\
    {} & {4/4} & {147} & {30} & {1} \\
    \multirow{-4}{*}{{\begin{tabular}[c]{@{}c@{}}LSQ\end{tabular}}} & {8/8} & {147} & {30} & {2.01} \\ \hline
    {} & {2/2} & {112} & {61} & {1.32} \\
    {} & {3/3} & {112} & {61} & {1.2} \\
    {} & {4/4} & {112} & {61} & {1.46} \\ 
    \multirow{-4}{*}{{\begin{tabular}[c]{@{}c@{}}OMPQ\end{tabular}}} & {8/8} & {112} & {61} & {1.74} \\ \hline
    {} & {2/2} & {113} & {61} & {1.32} \\
    {} & {3/3} & {113} & {61} & {1.2} \\
    {} & {4/4} & {113} & {61} & {1.46} \\
    \multirow{-4}{*}{{RAAD}} & {8/8} & {113} & {61} & {1.74} \\ \bottomrule[1.0pt] 
    \end{tabular}
    \caption{Comparing different PTQ methods and bit widths on the inference speed, GPU memory, and model parameters.} 
    \label{appendix_tab1}
\end{table}

In Table~\ref{appendix_tab2} and Table~\ref{appendix_tab2_2}, a comparison of the existing state-of-the-art IAD methods with POAD in terms of model size and inference time is presented, along with the detection strategies used by these methods. 

We believe that industrial defect methods suitable for edge devices should not only have low false negatives rate and false positives rate but also possess three key attributes: 1. Fast inference speed (high FPS), 2. Low GPU memory, and 3. Small model parameters. In Table~\ref{appendix_tab2}, it can be observed that the memory bank strategy using feature embeddings achieves the best results in image-level detection but also incurs a certain memory overhead. Reconstruction-based strategies perform better at the pixel level.

\begin{table}[!ht]
\centering

\setlength\tabcolsep{7pt}
    \begin{tabular}{l|ccc}
    \toprule[1.0pt]
    {Method} & {FPS} & {MEM(MB)} & {Params(M)} \\ \hline
    {EfficientAD-S} & {167} & {30.7} & {8.05}\\
    {PatchCore} & 25 & 267 & 68\\
    {RD4D} & 6 & 18 & 150 \\
    {SimpleNet}& 4 & 8 & 72\\
    {CPR}& 125 & 3226 & 2.88 \\ \hline
    {RAAD} & {113} & {61} & {1.46} \\ \bottomrule[1.0pt] 
    \end{tabular}
    \caption{Comparison of existing advanced IAD methods and RAAD in inference time, memory usage, and model parameters.} 
    \label{appendix_tab2}
\end{table}

\begin{table}[!ht]
\centering

\setlength\tabcolsep{6pt}
    \begin{tabular}{l|c|cc}
    \toprule[1.0pt]
    {Method} & strategy&AU-ROC &AU-PRO \\ \hline
    {EfficientAD-S} & T-S+AutoE& 96.98 & 91.38 \\
    {PatchCore} & Memory Bank& 99 & 93.5 \\
    {RD4D} & T-S& 98.5 & 93.9 \\
    {SimpleNet} & AD Synthesis & 98.1 & 92.9 \\
    {CPR} & Memory Bank& 99.7 & 97.8 \\ \hline
    {RAAD} & T-S+AutoE& 98.9 & 92.92 \\ \bottomrule[1.0pt] 
    \end{tabular}
    \caption{The advanced IAD method uses detection strategies and image-level detection accuracy Detection AU-ROC and pixel-level accuracy Segmentation AU-PRO.} 
    \label{appendix_tab2_2}
\end{table}
\begin{table}[!ht]
\centering

\setlength\tabcolsep{9pt}
    \begin{tabular}{l|cccc}
    \toprule[1.0pt]
    {Depth} & 28 & 40 & 64 & 100 \\ \hline
    {FPS} & 178 & 125 & 91 & 65 \\
    {Mem(MB)} & 9.6 & 11 & 14.25 & 18.8 \\
    {Params(M)} & 2.5 & 2.88 & 3.66 & 4..83 \\
    Det. AUROC & 89.11 & 98 & 92.3 & 80.97 \\
    Seg. AUPRO & 85.18 & 91.37 & 87.87 & 83.91
    \\ \bottomrule[1.0pt] 
    \end{tabular}
    \caption{Using Wide-ResNet of different depths on Inference FPS, GPU Memory, model parameters. And evaluate Detection AU-ROC and Segmentation AU-PRO on capsule category.} 
    \label{appendix_tab3}
\end{table}

\section{Comparison with models using transformer architecture}
We compared the Det. AU-ROC metrics on the MVTec-AD dataset with methods using Transformer architectures. It can be observed that Transformer-based methods show significant performance variation across different categories, whereas RAAD is more balanced. This demonstrates that RAAD has stronger adaptability and generalization across different categories, and its overall score is superior to other methods.

We also tested our method based on the FOD approach. As shown in Table 8, FOD-Quant represents the quantized FOD model. It is important to clarify that our method is based on a CNN model, and the attention mentioned in the text is an analogy, not equivalent to the attention mechanism in Transformers.
\begin{table*}
    \begin{center}
    
    \setlength\tabcolsep{8pt}
    \begin{tabular}{lccccc|c}
    \toprule[1.0pt]
    % \hline
    \multicolumn{2}{c|}{Category} & {\begin{tabular}[c]{@{}c@{}}InTra \\ (CVPR 2021)\end{tabular}} & {\begin{tabular}[c]{@{}c@{}}UniAD \\ (NeurIPS 2022)\end{tabular}} & {\begin{tabular}[c]{@{}c@{}}FOD \\ (ICCV 2023)\end{tabular}} & \begin{tabular}[c]{@{}c@{}}FOD\\ (Quant)\end{tabular} & {RAAD} \\ \hline
    \multicolumn{1}{l|}{} & \multicolumn{1}{c|}{{Carpet}} & {98.8} & {98.5} & {99.6} & {97.9} & {98.7} \\
    \multicolumn{1}{l|}{} & \multicolumn{1}{c|}{{Grid}} & {100} & {96.5} & {99.6} & {99.4} & {99.8} \\
    \multicolumn{1}{l|}{} & \multicolumn{1}{c|}{{Leather}} & {100} & {98.8} & {100} & {99.8} & {98.3} \\
    \multicolumn{1}{l|}{} & \multicolumn{1}{c|}{{Tile}} & {98.2} & {91.8} & {100} & {99.9} & {100} \\
    \multicolumn{1}{l|}{} & \multicolumn{1}{c|}{{Wood}} & {97.5} & {93.2} & {98.8} & {98.2} & {98.5} \\ \cline{2-7}  
    \multicolumn{1}{l|}{\multirow{-6}{*}{\rotatebox[origin=c]{90}{textures}}} & \multicolumn{1}{c|}{{avg.}} & {98.9} & {95.7} & {99.6} & {99.1} & {99.0} \\ \hline
    \multicolumn{1}{l|}{} & \multicolumn{1}{c|}{{Bottle}} & {100} & {98.1} & {100} & {99.8} & {100} \\
    \multicolumn{1}{l|}{} & \multicolumn{1}{c|}{{Cable}} & {70.3} & {97.3} & {98.4} & {98.5} & {97.7} \\
    \multicolumn{1}{l|}{} & \multicolumn{1}{c|}{{Capsule}} & {86.5} & {98.5} & {95.45} & {95.4} & {97.4} \\
    \multicolumn{1}{l|}{} & \multicolumn{1}{c|}{{Hazelnut}} & {95.7} & {98.1} & {100} & {100} & {99.7} \\
    \multicolumn{1}{l|}{} & \multicolumn{1}{c|}{{Metal\_nut}} & {96.9} & {94.8} & {99.9} & {98.1} & {98.8} \\
    \multicolumn{1}{l|}{} & \multicolumn{1}{c|}{{Pill}} & {90.2} & {95} & {94.2} & {95.0} & {98.0} \\
    \multicolumn{1}{l|}{} & \multicolumn{1}{c|}{{Screw}} & {95.7} & {98.3} & {94.7} & {90.7} & {98.5} \\
    \multicolumn{1}{l|}{} & \multicolumn{1}{c|}{{Toothbrush}} & {100} & {98.4} & {95.0} & {93.3} & {100} \\
    \multicolumn{1}{l|}{} & \multicolumn{1}{c|}{{Transistor}} & {95.7} & {97.9} & {99.75} & {99.5} & {100} \\
    \multicolumn{1}{l|}{} & \multicolumn{1}{c|}{{Zipper}} & {99.4} & {96.8} & {94.0} & {98.7} & {97.8} \\ \cline{2-7} 
    \multicolumn{1}{l|}{\multirow{-10}{*}{\rotatebox[origin=c]{90}{object}}} & \multicolumn{1}{c|}{{avg.}} & {93.0} & {97.3} & {97.1} & {96.9} & {98.8} \\ \hline
    \multicolumn{2}{l|}{avg. all category} & {95.0} & {96.8} & {97.9} & {92.9} & {98.9} \\ 
    % \hline
    \bottomrule[1.0pt]
    \end{tabular}
    \caption{
    Compared the Det. AU-ROC metric on the MVTec-AD dataset using Transformer architecture methods, ``FOD-Quant'': Quantitative evaluation results of the FOD.
    } 
    \end{center}
\end{table*}

\begin{figure*}
 \includegraphics[width=1\linewidth]{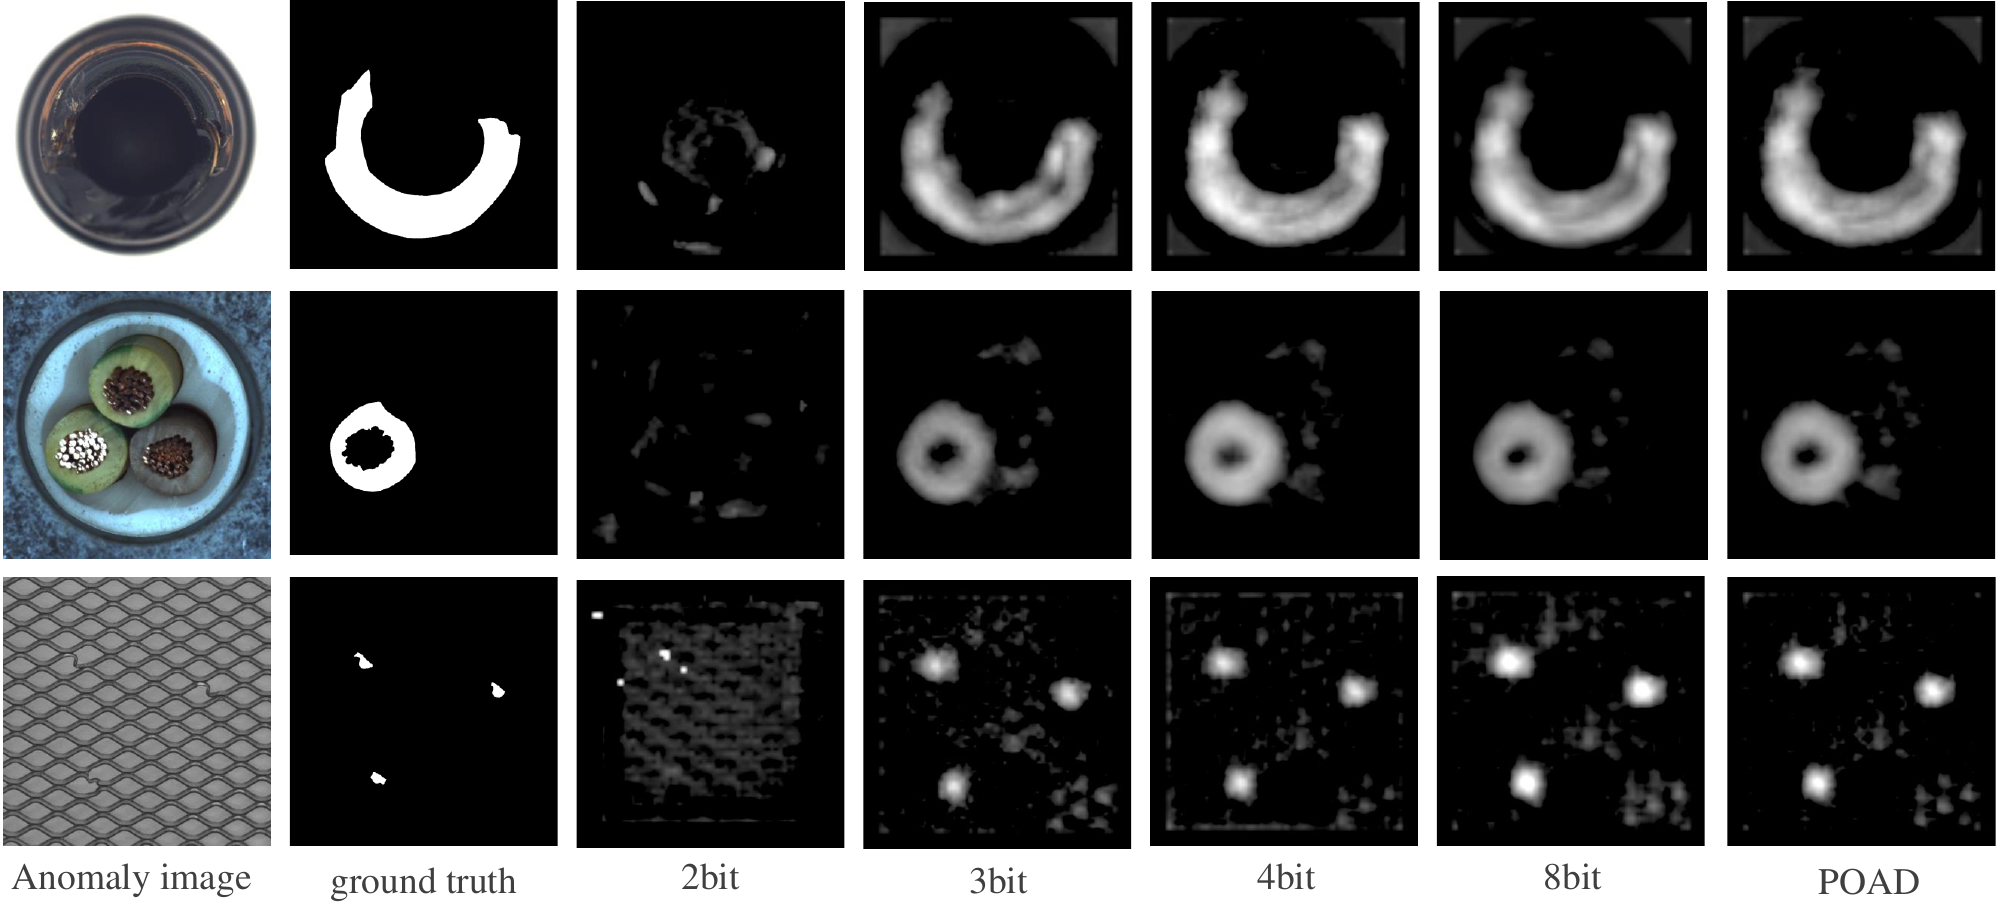}
 \caption{Visualization of anomaly maps on MVTec AD with baseline and different PTQ method.} 
 \label{appendix_fig1} 
\end{figure*}
\section{Using Different Networks}
In Table~\ref{appendix_tab3}, the impact of replacing the POAD feature extraction network PDN with Wide-ResNet of different depths on model accuracy, model size, and inference time is demonstrated. Since the depth of Wide-ResNet needs to satisfy $(depth-4)\%6=0$, we choose depths of 28, 40, 64, and 100.

\section{Qualitative Results}
We visualized the results on the MVTec-AD dataset, as shown in Figure~\ref{appendix_fig1}, demonstrating the impact of our method using different quantization bit widths on anomaly maps. Moreover, in Figure~\ref{appendix_fig2}, comparing the different PTQ methods on MVTec AD and MVTec LOCO-AD. The baseline results are obtained using EfficientAD-S~\cite{batzner2024efficientad}.

\begin{figure}
 \includegraphics[width=1\linewidth]{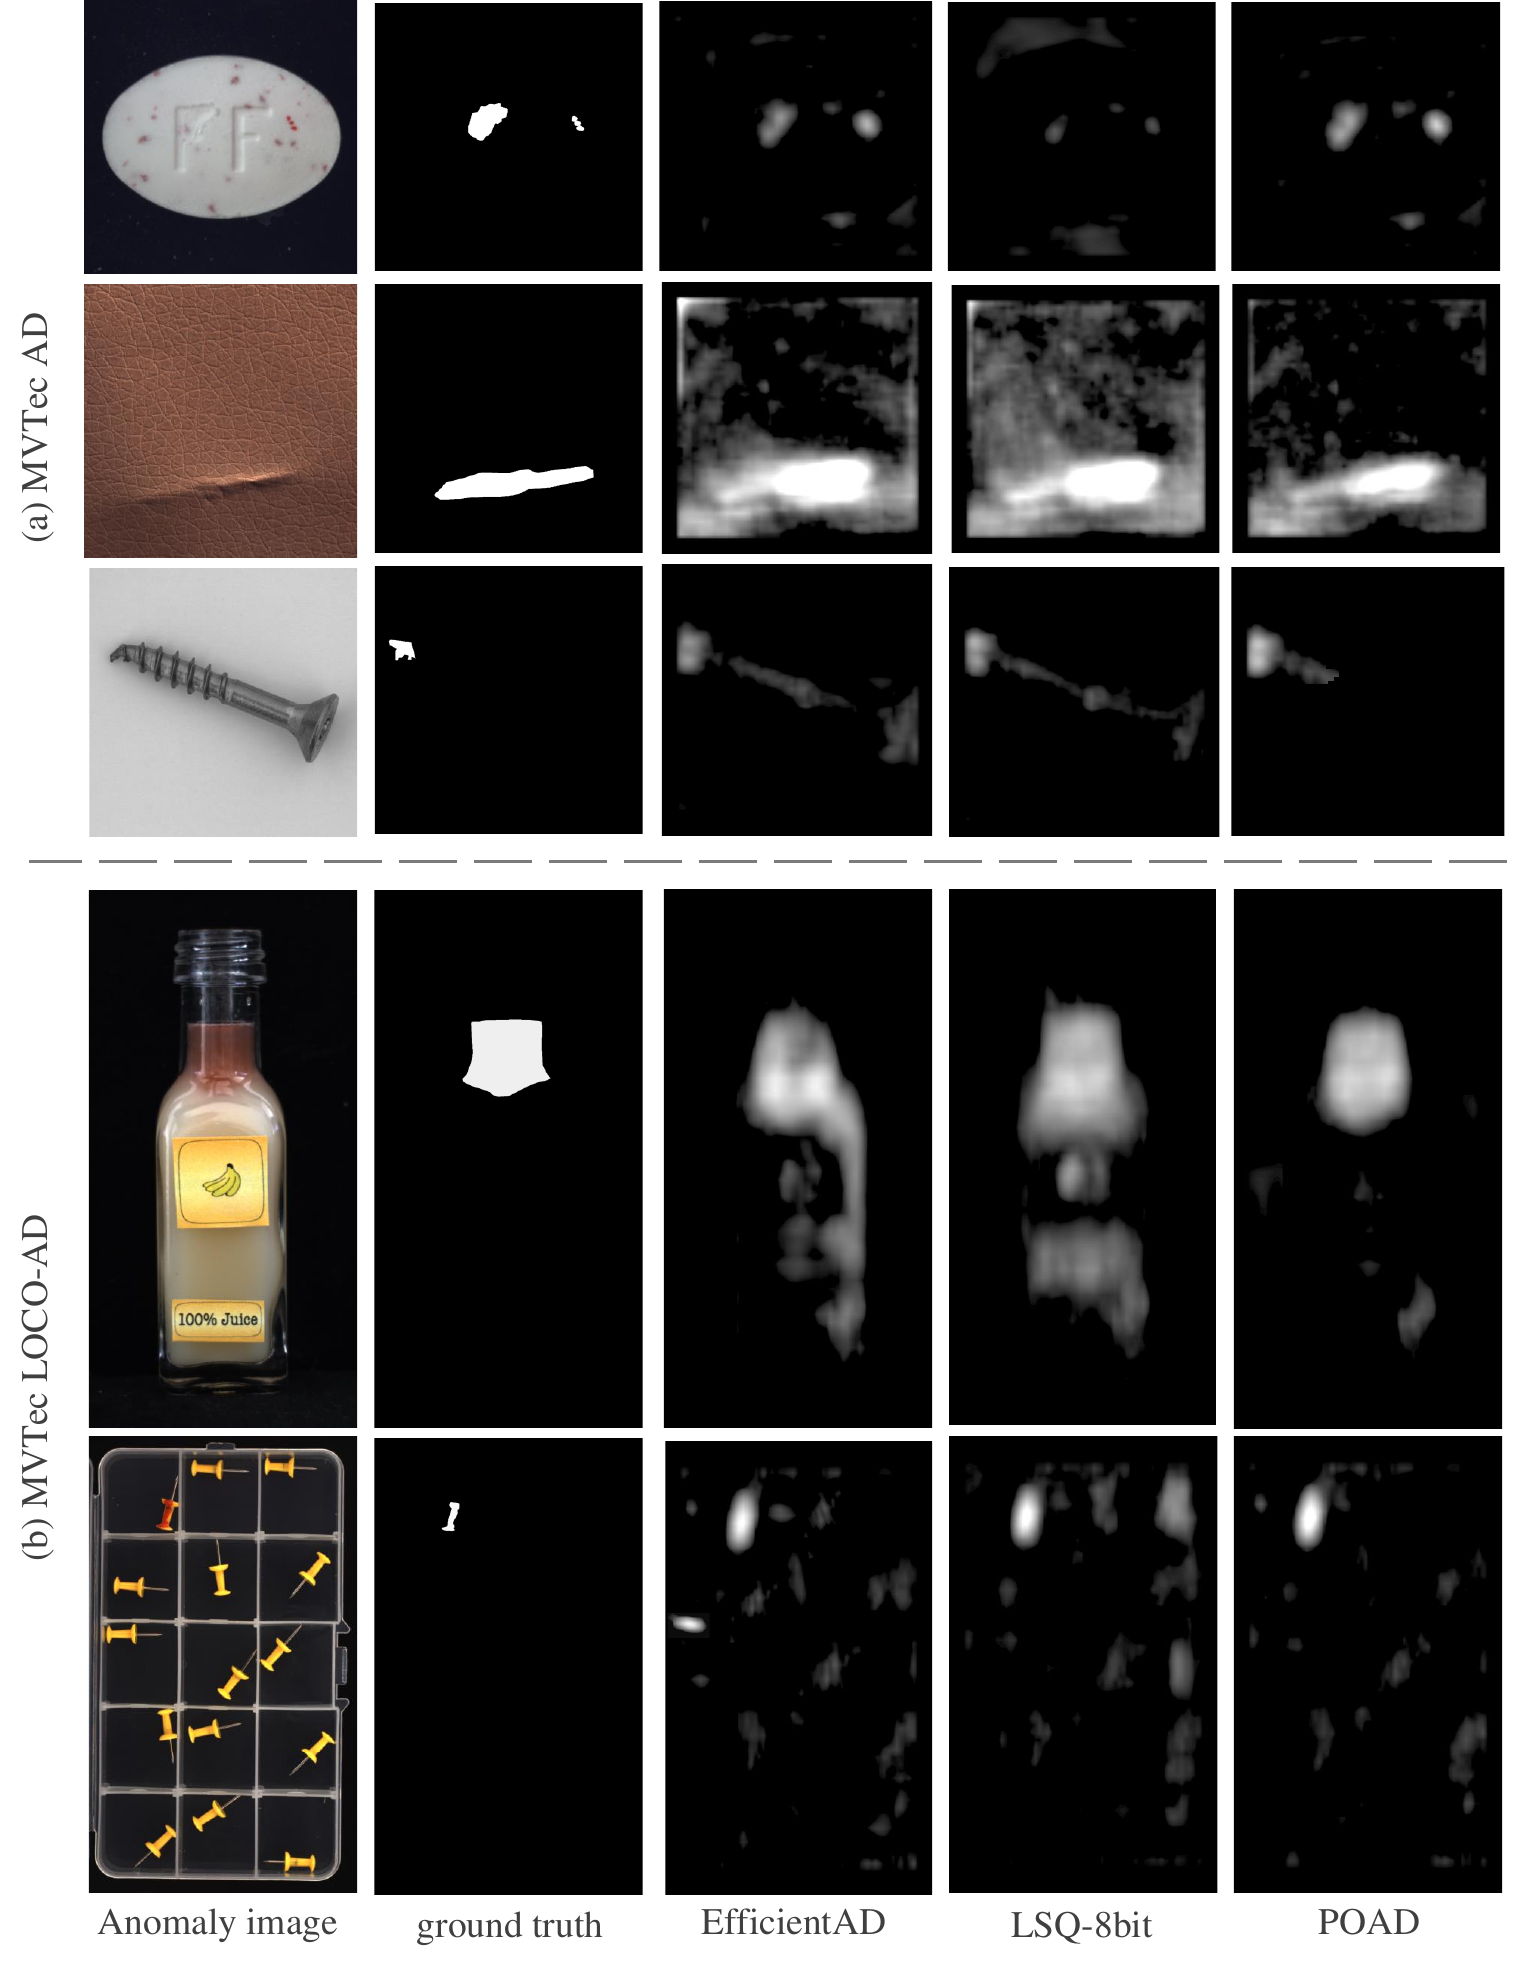}
 \caption{Visualization of anomaly maps on MVTec AD and MVTec LOCO-AD with} 
 \label{appendix_fig2} 
\end{figure}

\section{Future Works}
Unlike model compression, our approach employs model quantization not with the aim of reducing model size, but rather to achieve dimensionality reduction at the precision level. Some industrial anomaly detection efforts currently utilize model quantization during deployment to reduce model size while maintaining certain accuracy levels. For instance, CPR~\cite{li2023target} has achieved 1016 FPS using TensorRT on NVIDIA RTX4090 GPU.

In future work, we intend to propose a post-training quantization method specifically designed for the industrial anomaly detection domain, utilizing PyTorch. This method would be applied to post-training models to reduce model size while maintaining or even enhancing model accuracy.

Additionally, we aim to conduct experiments on the more challenging IAD dataset. Currently, most state-of-the-art methods have reached saturation (AUROC exceeding 99\%) on mainstream datasets like MVTec, making it difficult to distinguish between methods, which leads to unsatisfactory performance in practical applications. A recently introduced dataset, Real-IAD~\cite{wang2024real}, has garnered attention due to its large scale, real-world context, and multi-view nature. In future work, we plan to experiment with this dataset.
