# Supplementary material for: Breaking the Bias: Recalibrating the Attention of Industrial Anomaly Detection
Source: arXiv:2412.08189 source file (2024-12-11)
Supplement: Supplementary file 3 [file tab5_appendix_1.tex]

\begin{table}[!ht]
\centering

\setlength\tabcolsep{6pt}
    \begin{tabular}{c|cccc}
    \toprule[1.0pt]
    {Method} & {W/A} & {FPS} & {Mem(MB)} & {Params(M)} \\ \hline 
    {baseline} & {32/32} & \multicolumn{1}{c}{{167}} & {30.7} & {8.05} \\ \hline
    {} & {2/2} & \multicolumn{1}{c}{{147}} & {30} & {0.5} \\
    {} & {3/3} & \multicolumn{1}{c}{{147}} & {30} & {0.75} \\
    {} & {4/4} & {147} & {30} & {1} \\
    \multirow{-4}{*}{{\begin{tabular}[c]{@{}c@{}}LSQ\end{tabular}}} & {8/8} & {147} & {30} & {2.01} \\ \hline
    {} & {2/2} & {112} & {61} & {1.32} \\
    {} & {3/3} & {112} & {61} & {1.2} \\
    {} & {4/4} & {112} & {61} & {1.46} \\ 
    \multirow{-4}{*}{{\begin{tabular}[c]{@{}c@{}}OMPQ\end{tabular}}} & {8/8} & {112} & {61} & {1.74} \\ \hline
    {} & {2/2} & {113} & {61} & {1.32} \\
    {} & {3/3} & {113} & {61} & {1.2} \\
    {} & {4/4} & {113} & {61} & {1.46} \\
    \multirow{-4}{*}{{RAAD}} & {8/8} & {113} & {61} & {1.74} \\ \bottomrule[1.0pt] 
    \end{tabular}
    \caption{Comparing different PTQ methods and bit widths on the inference speed, GPU memory, and model parameters.} 
    \label{appendix_tab1}
\end{table}
