# Supplementary material for: Breaking the Bias: Recalibrating the Attention of Industrial Anomaly Detection
Source: arXiv:2412.08189 source file (2024-12-11)
Supplement: Supplementary file 4 [file tab6_appendix_2.tex]

\begin{table}[!ht]
\centering

\setlength\tabcolsep{7pt}
    \begin{tabular}{l|ccc}
    \toprule[1.0pt]
    {Method} & {FPS} & {MEM(MB)} & {Params(M)} \\ \hline
    {EfficientAD-S} & {167} & {30.7} & {8.05}\\
    {PatchCore} & 25 & 267 & 68\\
    {RD4D} & 6 & 18 & 150 \\
    {SimpleNet}& 4 & 8 & 72\\
    {CPR}& 125 & 3226 & 2.88 \\ \hline
    {RAAD} & {113} & {61} & {1.46} \\ \bottomrule[1.0pt] 
    \end{tabular}
    \caption{Comparison of existing advanced IAD methods and RAAD in inference time, memory usage, and model parameters.} 
    \label{appendix_tab2}
\end{table}

\begin{table}[!ht]
\centering

\setlength\tabcolsep{6pt}
    \begin{tabular}{l|c|cc}
    \toprule[1.0pt]
    {Method} & strategy&AU-ROC &AU-PRO \\ \hline
    {EfficientAD-S} & T-S+AutoE& 96.98 & 91.38 \\
    {PatchCore} & Memory Bank& 99 & 93.5 \\
    {RD4D} & T-S& 98.5 & 93.9 \\
    {SimpleNet} & AD Synthesis & 98.1 & 92.9 \\
    {CPR} & Memory Bank& 99.7 & 97.8 \\ \hline
    {RAAD} & T-S+AutoE& 98.9 & 92.92 \\ \bottomrule[1.0pt] 
    \end{tabular}
    \caption{The advanced IAD method uses detection strategies and image-level detection accuracy Detection AU-ROC and pixel-level accuracy Segmentation AU-PRO.} 
    \label{appendix_tab2_2}
\end{table}
