# Supplementary material for: Breaking the Bias: Recalibrating the Attention of Industrial Anomaly Detection
Source: arXiv:2412.08189 source file (2024-12-11)
Supplement: Supplementary file 5 [file tab7_appendix_3.tex]

\begin{table}[!ht]
\centering

\setlength\tabcolsep{9pt}
    \begin{tabular}{l|cccc}
    \toprule[1.0pt]
    {Depth} & 28 & 40 & 64 & 100 \\ \hline
    {FPS} & 178 & 125 & 91 & 65 \\
    {Mem(MB)} & 9.6 & 11 & 14.25 & 18.8 \\
    {Params(M)} & 2.5 & 2.88 & 3.66 & 4..83 \\
    Det. AUROC & 89.11 & 98 & 92.3 & 80.97 \\
    Seg. AUPRO & 85.18 & 91.37 & 87.87 & 83.91
    \\ \bottomrule[1.0pt] 
    \end{tabular}
    \caption{Using Wide-ResNet of different depths on Inference FPS, GPU Memory, model parameters. And evaluate Detection AU-ROC and Segmentation AU-PRO on capsule category.} 
    \label{appendix_tab3}
\end{table}
