# Supplementary material for: Breaking the Bias: Recalibrating the Attention of Industrial Anomaly Detection
Source: arXiv:2412.08189 source file (2024-12-11)
Supplement: Supplementary file 6 [file tab8_appendix_4.tex]

\begin{table*}
    \begin{center}
    
    \setlength\tabcolsep{8pt}
    \begin{tabular}{lccccc|c}
    \toprule[1.0pt]
    % \hline
    \multicolumn{2}{c|}{Category} & {\begin{tabular}[c]{@{}c@{}}InTra \\ (CVPR 2021)\end{tabular}} & {\begin{tabular}[c]{@{}c@{}}UniAD \\ (NeurIPS 2022)\end{tabular}} & {\begin{tabular}[c]{@{}c@{}}FOD \\ (ICCV 2023)\end{tabular}} & \begin{tabular}[c]{@{}c@{}}FOD\\ (Quant)\end{tabular} & {RAAD} \\ \hline
    \multicolumn{1}{l|}{} & \multicolumn{1}{c|}{{Carpet}} & {98.8} & {98.5} & {99.6} & {97.9} & {98.7} \\
    \multicolumn{1}{l|}{} & \multicolumn{1}{c|}{{Grid}} & {100} & {96.5} & {99.6} & {99.4} & {99.8} \\
    \multicolumn{1}{l|}{} & \multicolumn{1}{c|}{{Leather}} & {100} & {98.8} & {100} & {99.8} & {98.3} \\
    \multicolumn{1}{l|}{} & \multicolumn{1}{c|}{{Tile}} & {98.2} & {91.8} & {100} & {99.9} & {100} \\
    \multicolumn{1}{l|}{} & \multicolumn{1}{c|}{{Wood}} & {97.5} & {93.2} & {98.8} & {98.2} & {98.5} \\ \cline{2-7}  
    \multicolumn{1}{l|}{\multirow{-6}{*}{\rotatebox[origin=c]{90}{textures}}} & \multicolumn{1}{c|}{{avg.}} & {98.9} & {95.7} & {99.6} & {99.1} & {99.0} \\ \hline
    \multicolumn{1}{l|}{} & \multicolumn{1}{c|}{{Bottle}} & {100} & {98.1} & {100} & {99.8} & {100} \\
    \multicolumn{1}{l|}{} & \multicolumn{1}{c|}{{Cable}} & {70.3} & {97.3} & {98.4} & {98.5} & {97.7} \\
    \multicolumn{1}{l|}{} & \multicolumn{1}{c|}{{Capsule}} & {86.5} & {98.5} & {95.45} & {95.4} & {97.4} \\
    \multicolumn{1}{l|}{} & \multicolumn{1}{c|}{{Hazelnut}} & {95.7} & {98.1} & {100} & {100} & {99.7} \\
    \multicolumn{1}{l|}{} & \multicolumn{1}{c|}{{Metal\_nut}} & {96.9} & {94.8} & {99.9} & {98.1} & {98.8} \\
    \multicolumn{1}{l|}{} & \multicolumn{1}{c|}{{Pill}} & {90.2} & {95} & {94.2} & {95.0} & {98.0} \\
    \multicolumn{1}{l|}{} & \multicolumn{1}{c|}{{Screw}} & {95.7} & {98.3} & {94.7} & {90.7} & {98.5} \\
    \multicolumn{1}{l|}{} & \multicolumn{1}{c|}{{Toothbrush}} & {100} & {98.4} & {95.0} & {93.3} & {100} \\
    \multicolumn{1}{l|}{} & \multicolumn{1}{c|}{{Transistor}} & {95.7} & {97.9} & {99.75} & {99.5} & {100} \\
    \multicolumn{1}{l|}{} & \multicolumn{1}{c|}{{Zipper}} & {99.4} & {96.8} & {94.0} & {98.7} & {97.8} \\ \cline{2-7} 
    \multicolumn{1}{l|}{\multirow{-10}{*}{\rotatebox[origin=c]{90}{object}}} & \multicolumn{1}{c|}{{avg.}} & {93.0} & {97.3} & {97.1} & {96.9} & {98.8} \\ \hline
    \multicolumn{2}{l|}{avg. all category} & {95.0} & {96.8} & {97.9} & {92.9} & {98.9} \\ 
    % \hline
    \bottomrule[1.0pt]
    \end{tabular}
    \caption{
    Compared the Det. AU-ROC metric on the MVTec-AD dataset using Transformer architecture methods, ``FOD-Quant'': Quantitative evaluation results of the FOD.
    } 
    \end{center}
\end{table*}
